# Supplementary material for: RuozhiBench: Evaluating LLMs with Logical Fallacies and Misleading Premises
Source: arXiv:2502.13125 source file (2025-02-18)
Supplement: Supplementary file 1 [file data_structure.tex]

\UseRawInputEncoding
In \dataset, each data entry contains the question, the language category of the question, the attribute of the question, and the irrationality analysis of the question. And the question attribute is limited to two categories: tricky or not tricky. The irrationality analysis means a detailed explanation highlighting the logical flaws or unrealistic assumptions present in the tricky question. In the following code block, there are two samples in \dataset, including one tricky sample and one normal sample.

\begin{lstlisting}[language=JSON]
{
    "question": "Why are there spaces between words in English, but no need to pause between words when reading a sentence?",
    "language": "en",
    "troll": 1,
    "irrationality": "Reading naturally includes brief pauses between words even if they are not explicitly marked, and spaces in written language help visually identify word boundaries."
}
\end{lstlisting}
