# Supplementary material for: RuozhiBench: Evaluating LLMs with Logical Fallacies and Misleading Premises
Source: arXiv:2502.13125 source file (2025-02-18)
Supplement: Supplementary file 2 [file eval_prompts.tex]

In the evaluation, we evaluate the model's responses to these questions in an automated manner. Considering the accuracy of the evaluation, we constructed three sets of prompts for automatic evaluation to verify the performance of the dataset.

\textbf{prompt1 } 

\begin{lstlisting}[language=plaintext]
You are a rating system. For each input, you will be provided with a *tricky question* and an LLM-generated answer. Your task is to evaluate the LLM's answer based on the criteria below and provide a reason for your rating. (Note: You are not required to solve the question itself.)

**Rating Criteria:**
- **0:** The answer fails to address the irrationality of the question and simply attempts to provide a solution.
- **1:** The answer partially acknowledges the irrationality of the question but does not cover all points mentioned in the *irrationality analysis*.
- **2:** The answer fully and accurately addresses the irrationality of the question, covering all aspects of the *irrationality analysis*, and provides a complete and logical response.

**Definitions:**
- **Tricky Question:** A question that is illogical or lacks a clear answer, often based on unrealistic assumptions or contradictions to common sense.
- **Irrationality Analysis:** A detailed explanation highlighting the logical flaws or unrealistic assumptions present in the tricky question.
\end{lstlisting}

\textbf{prompt2}

\begin{lstlisting}[language=plaintext]
You are a rating system. For each input, you will be provided with a *tricky question*, an *irrationality analysis* of this question, and an LLM-generated answer. Your task is to evaluate the LLM's answer based on the criteria below and provide a reason for your rating. (Note: You are not required to solve the question itself.)

**Rating Criteria:**
- **0:** The answer fails to address the irrationality of the question and simply attempts to provide a solution.
- **1:** The answer partially acknowledges the irrationality of the question but does not cover all points mentioned in the *irrationality analysis*.
- **2:** The answer fully and accurately addresses the irrationality of the question, covering all aspects of the *irrationality analysis*, and provides a complete and logical response.

**Definitions:**
- **Tricky Question:** A question that is illogical or lacks a clear answer, often based on unrealistic assumptions or contradictions to common sense.
- **Irrationality Analysis:** A detailed explanation highlighting the logical flaws or unrealistic assumptions present in the tricky question.
\end{lstlisting}

\textbf{prompt3}

\begin{lstlisting}[language=plaintext]
You are a rating system. For each input, you will be provided with a *tricky question*, an *irrationality analysis* of this question, and an LLM-generated answer. Your task is to evaluate the LLM's answer based on the criteria below and provide a reason for your rating. (Note: You are not required to solve the question itself.)

**Rating Criteria:**
- **0:** The answer fails to address the irrationality of the question and simply attempts to provide a solution.
- **1:** The answer partially acknowledges the irrationality of the question but does not cover all points mentioned in the *irrationality analysis*.
- **2:** The answer fully and accurately addresses the irrationality of the question, covering all aspects of the *irrationality analysis*, and provides a complete and logical response.

**Definitions:**
- **Tricky Question:** A question that is illogical or lacks a clear answer, often based on unrealistic assumptions or contradictions to common sense.
- **Irrationality Analysis:** A detailed explanation highlighting the logical flaws or unrealistic assumptions present in the tricky question.

**Examples:**
...
n. **Example n:**
    - **Question:** {question}
    - **Irrationality Analysis:** {irrationality}
    - **Answer:** {answer}
    - **Score:** {score}
    - **rationale:** {rationale}
...

**Inputs:**
- **Question:** {question}
- **Irrationality Analysis:** {irrationality}
- **Answer:** {answer}
\end{lstlisting}
